# Supplementary material for: Primordial Bounce-Inflation Scenario to Alleviate Cosmological Tensions and Lensing Anomaly
Source: arXiv:2409.04027 source file (2025-02-19)
Supplement: Supplementary file 1 [file Sup_Mat.pdf]

# Supplementary material for "Primordial Bounce-Inflation Scenario to Alleviate Cosmological Tensions and Lensing Anomaly"

Hao-Hao Li[a,1], Xin-zhe Zhang[a,2], Taotao Qiu[a,3]
[a]*School of Physics, Huazhong University of Science and Technology, Wuhan, 430074, China*

This Supplementary Material includes a parameterized background of the Bounce-Inflation scenario and the calculations of the primordial power spectrum in Section A. Section B consists of the mean value and 68% limits of cosmological parameters for all cases we considered. Section C shows the constraints of the cosmological parameters when we add a prior of $\tau_{reio}$.

## A. Bounce-Inflation

Firstly, we parameterize the background of the Bounce-Inflation (BI) scenario where the scale factor follows

$$a = \begin{cases} a_{con}\left(\tilde{\eta}_{B-} - \eta\right)^{\frac{1}{\epsilon_c - 1}} & \eta < \eta_{B-}, \\ a_B\left[1 + \frac{\alpha}{2}\left(\eta - \eta_B\right)^2\right] & \eta_{B-} \leq \eta \leq \eta_{B+} , \\ a_{exp}\left(\tilde{\eta}_{B+} - \eta\right)^{\frac{1}{\epsilon_e - 1}} & \eta > \eta_{B+}, \end{cases} \tag{1}$$

with $\tilde{\eta}_{B-} \equiv \eta_{B-} - \left[\left(\epsilon_c - 1\right)\mathcal{H}_{con}\right]^{-1}$, $\tilde{\eta}_{B+} \equiv \eta_{B+} - \left[\left(\epsilon_e - 1\right)\mathcal{H}_{exp}\right]^{-1}$. Here, $\eta$ is the conformal time and $\eta_{B-}$ $(\eta_{B+})$ is the beginning (ending) of the bouncing phase, $a_B$ is the scale factor at the bouncing point $\eta_B$, $\mathcal{H}_{con}\,(\mathcal{H}_{exp})$ is the conformal Hubble parameter at $\eta_{B-}\,(\eta_{B+})$, and $\epsilon_c\,(\epsilon_e)$ is the slow-roll parameter in the contracting(inflationary) phase. The three lines in parameterization (1) represent the contracting, bouncing, and expanding phases of the primordial universe, respectively. Moreover, to avoid the contracting anisotropy problem [1–7], we require that $\epsilon_c$ is larger than 3, which means that the parameter of the equation of state $w$ in the contracting phase is larger than 1 from the relationship $\epsilon_c = 3\left(1 + w\right)/2$.

The curvature perturbation $\mathcal{R}$ is governed by the Mukhanov-Sasaki equation:

$$u_k'' + \left(c_s^2 k^2 - \frac{z''}{z}\right) u_k = 0, \tag{2}$$

with $u_k \equiv z\mathcal{R}$, $z \equiv a\sqrt{Q}/c_s$. The variable $Q$ can be calculated based on the effective field theory of cosmology [8–11]. The scale factor $a$ and the slow-roll parameter $\epsilon$ in each phase are given by Eq. (1), while the solutions of different phases are connected using the matching

[1] e-mail: lihaohao23@hust.edu.cn
[2] e-mail: zincz@hust.edu.cn
[3] e-mail: qiutt@hust.edu.cn

conditions [8]. We follow [8] to write down the primordial power spectrum of BI

$$P_{\mathcal{R}} = \frac{H_{exp}^2}{8\pi^2 M_p^2 \epsilon_e} \left(\frac{k}{k_*}\right)^{3-2\nu_e} |C_1 - C_2|^2, \tag{3}$$

where $\nu_e = \frac{\epsilon_e - 3}{2(\epsilon_e - 1)}$,

$$\begin{aligned} C_1 = &-ie^{i\nu_{c1}\pi}\sqrt{\frac{\tilde{\mathcal{H}}_e}{\tilde{\mathcal{H}}_c}}\pi^{3/2}\sin(l\Delta\eta_B)\Bigg\{k\left[H^{(1)}_{\nu_c+1}\left(\frac{k}{\tilde{\mathcal{H}}_c}\right) - H^{(1)}_{\nu_c-1}\left(\frac{k}{\tilde{\mathcal{H}}_c}\right)\right]\left[k\left(H^{(2)}_{\nu_e+1}\left(\frac{k}{\tilde{\mathcal{H}}_e}\right)\right.\right. \\ &\left.\left. - H^{(2)}_{\nu_e-1}\left(\frac{k}{\tilde{\mathcal{H}}_e}\right)\right) - \left(\tilde{\mathcal{H}}_e + 2l\cot(l\Delta\eta_B)\right)H^{(2)}_{\nu_e}\left(\frac{k}{\tilde{\mathcal{H}}_e}\right)\right] + H^{(1)}_{\nu_c}\left(\frac{k}{\tilde{\mathcal{H}}_c}\right)\Bigg[\tilde{\mathcal{H}}_e\tilde{\mathcal{H}}_c + 4l^2 \\ &+ 2\left(\tilde{\mathcal{H}}_c - \tilde{\mathcal{H}}_e\right)l\cot(l\Delta\eta_B)\Bigg]H^{(2)}_{\nu_e}\left(\frac{k}{\tilde{\mathcal{H}}_e}\right) + k\left(2l\cot(l\Delta\eta_B) - \tilde{\mathcal{H}}_c\right)\left(H^{(2)}_{\nu_e+1}\left(\frac{k}{\tilde{\mathcal{H}}_e}\right)\right. \\ &\left. - H^{(2)}_{\nu_e-1}\left(\frac{k}{\tilde{\mathcal{H}}_e}\right)\right)\Bigg\}\Bigg/\left[16l\tilde{\mathcal{H}}_e + 8lk\pi\left(J_{\nu_e}\left(\frac{k}{\tilde{\mathcal{H}}_e}\right)Y_{\nu_e-1}\left(\frac{k}{\tilde{\mathcal{H}}_e}\right) - J_{\nu_e-1}\left(\frac{k}{\tilde{\mathcal{H}}_e}\right)Y_{\nu_e}\left(\frac{k}{\tilde{\mathcal{H}}_e}\right)\right)\right] \end{aligned}, \tag{4}$$

and

$$\begin{aligned} C_2 = &\, ie^{i\nu_{c1}\pi}\sqrt{\frac{\tilde{\mathcal{H}}_e}{\tilde{\mathcal{H}}_c}}\pi^{3/2}\sin(l\Delta\eta_B)\Bigg\{k\left[H^{(1)}_{\nu_c+1}\left(\frac{k}{\tilde{\mathcal{H}}_c}\right) - H^{(1)}_{\nu_c-1}\left(\frac{k}{\tilde{\mathcal{H}}_c}\right)\right]\left[k\left(H^{(1)}_{\nu_e+1}\left(\frac{k}{\tilde{\mathcal{H}}_e}\right)\right.\right. \\ &\left.\left. - H^{(1)}_{\nu_e-1}\left(\frac{k}{\tilde{\mathcal{H}}_e}\right)\right) - \left(\tilde{\mathcal{H}}_e + 2l\cot(l\Delta\eta_B)\right)H^{(1)}_{\nu_e}\left(\frac{k}{\tilde{\mathcal{H}}_e}\right)\right] + H^{(1)}_{\nu_c}\left(\frac{k}{\tilde{\mathcal{H}}_c}\right)\Bigg[\tilde{\mathcal{H}}_e\tilde{\mathcal{H}}_c + 4l^2 \\ &+ 2\left(\tilde{\mathcal{H}}_c - \tilde{\mathcal{H}}_e\right)l\cot(l\Delta\eta_B)\Bigg]H^{(1)}_{\nu_e}\left(\frac{k}{\tilde{\mathcal{H}}_e}\right) + k\left(2l\cot(l\Delta\eta_B) - \tilde{\mathcal{H}}_c\right)\left(H^{(1)}_{\nu_e+1}\left(\frac{k}{\tilde{\mathcal{H}}_e}\right)\right. \\ &\left. - H^{(1)}_{\nu_e-1}\left(\frac{k}{\tilde{\mathcal{H}}_e}\right)\right)\Bigg\}\Bigg/\left[16l\tilde{\mathcal{H}}_e + 8lk\pi\left(J_{\nu_e}\left(\frac{k}{\tilde{\mathcal{H}}_e}\right)Y_{\nu_e-1}\left(\frac{k}{\tilde{\mathcal{H}}_e}\right) - J_{\nu_e-1}\left(\frac{k}{\tilde{\mathcal{H}}_e}\right)Y_{\nu_e}\left(\frac{k}{\tilde{\mathcal{H}}_e}\right)\right)\right] \end{aligned}, \tag{5}$$

with $\tilde{\mathcal{H}}_c = \mathcal{H}_{con} - \epsilon_c\mathcal{H}_{con}$, $\tilde{\mathcal{H}}_e = \mathcal{H}_{exp} - \epsilon_e\mathcal{H}_{exp}$, $\nu_c = (3-\epsilon_c)/[2(1-\epsilon_c)]$, $\nu_{c1} = (\epsilon_c - 2)/[2(\epsilon_c - 1)]$, $\nu_e = (3-\epsilon_e)/[2(1-\epsilon_e)]$, $\Delta\eta_B = \eta_{B+} - \eta_{B-}$, $l^2 = \bar{c}_s^2 k^2 - (\alpha - \chi)a_B^2$, $H^{(1)}$ and $H^{(2)}$ are the first and the second Hankel function, $J$ and $Y$ represent the first and the second Bessel function. Thus, five free parameters can describe the primordial power spectrums, that is, $\epsilon_c$, $\epsilon_e$, $\mathcal{H}_{con}$, $\mathcal{H}_{exp}$ and $\Delta\eta_B$. For the limit $k \gg \mathcal{H}_{exp}(\mathcal{H}_{con})$ and $l = k$, we have the approximation of $|C_1 - C_2|^2$ as

$$\begin{aligned} &|C_1 - C_2|^2 \simeq \\ &\quad \left[4\tilde{\mathcal{H}}_e^2\pi\left(4 + \frac{\Delta\tilde{\mathcal{H}}}{k}\cos\left[2\left(\Delta\eta_B + \frac{1}{\tilde{\mathcal{H}}_e}\right)k\right] + \frac{\Delta\tilde{\mathcal{H}}}{k}\cos\left(\frac{2k}{\tilde{\mathcal{H}}_e}\right)\right)\right]\Bigg/\left[\left(2\tilde{\mathcal{H}}_e\right.\right. \\ &\quad \left.\left. + k\pi J_{\nu_e}\left(\frac{k}{\tilde{\mathcal{H}}_e}\right)Y_{\nu_e-1}\left(\frac{k}{\tilde{\mathcal{H}}_e}\right) - k\pi J_{\nu_e-1}\left(\frac{k}{\tilde{\mathcal{H}}_e}\right)Y_{\nu_e}\left(\frac{k}{\tilde{\mathcal{H}}_e}\right)\right)^2\right], \end{aligned} \tag{6}$$

where $\Delta\tilde{\mathcal{H}} \equiv \tilde{\mathcal{H}}_e - \tilde{\mathcal{H}}_c$, and for the small $k$, $|C_1 - C_2|^2 \sim k^{2\epsilon_c/(\epsilon_c - 1)}$.

In the BI scenario, there is an inflationary stage at the beginning of the expanding phase. During inflation, we can use the asymptotic expressions of Hankel and Bessel functions when the argument is much larger than unity. Thus, we have $|C_1 - C_2|^2 \simeq 1$ for large $k$ and the primordial power spectrum can be parameterized as

$$P_{\mathcal{R},I} = A_s \left(\frac{k}{k_*}\right)^{n_s-1} . \tag{7}$$

The subscript "$I$" means the inflationary stage of the BI. $A_s$ is the scalar perturbation amplitude, $n_s$ is the spectral index, and the pivot scale $k_* = 0.05\text{Mpc}^{-1}$ for Planck satellite. Notice that $A_s$ and $n_s$ can be derived from the five free parameters $\{\mathcal{H}_{con}, \mathcal{H}_{exp}, \Delta\eta_B, \epsilon_c, \epsilon_e\}$ in Eq. (3).

| Params | P18 (BI) | P18 (BI+$A_L$) | P18+SPT3G (BI) | P18+SPT3G (BI+$A_L$) |
|---|---|---|---|---|
| $\boldsymbol{\epsilon_c}$ | $4.2^{+1.6}_{-1.2}$ | $7.7^{+2.0}_{-3.1}$ | $3.42^{+0.19}_{-0.34}$ | $4.10 \pm 0.16$ |
| $\mathbf{10^3}\boldsymbol{\epsilon_e}$ | $9.86^{+1.20}_{-0.59}$ | $9.57^{+0.97}_{-1.30}$ | $8.16 \pm 0.27$ | $7.97 \pm 0.18$ |
| $\mathbf{10^4}\boldsymbol{\mathcal{H}_{con}}$ | $-3.93^{+1.00}_{-0.84}$ | $-1.30^{+1.20}_{-0.38}$ | $-4.61^{+0.94}_{-0.75}$ | $-4.59 \pm 0.18$ |
| $\mathbf{10^5}\boldsymbol{\mathcal{H}_{exp}}$ | $4.58^{+0.20}_{-0.13}$ | $4.44 \pm 0.22$ | $4.168 \pm 0.076$ | $4.055 \pm 0.056$ |
| $\boldsymbol{\Delta\eta_B}$ | $4.2^{+1.4}_{-1.0}$ | $1.9^{+2.5}_{-1.8}$ | $2.62 \pm 0.20$ | $0.64^{+0.26}_{-0.14}$ |

TABLE I: Parameters (Mean and 68% limits) of the primordial power spectrum of BI with reduced Planck mass $M_P = 1$.

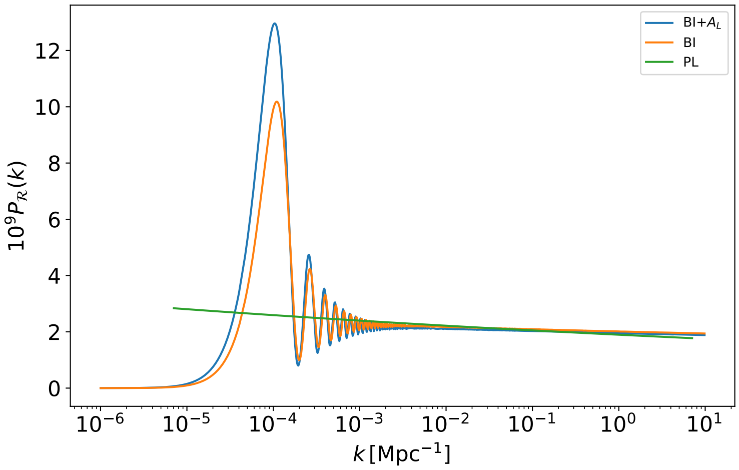


FIG. 1: The primordial power spectra with limits of P18 data sets based on the $\Lambda$CDM (BI), the extended $\Lambda$CDM (BI) + $A_L$ and $\Lambda$CDM (PL). The fiducial parameters of $\Lambda$CDM (PL) is the same as Planck-2018 results [12].

We consider $\Lambda$CDM (BI) and the extended version $\Lambda$CDM (BI) + $A_L$ using P18 and P18+SPT3G data to restrict the parameters of our BI model. The results are shown in TABLE I. The slow-roll parameter of the contracting phase $\epsilon_c > 3$ while that of the inflationary stage is in the order of $10^{-2}$. The energy scales represented by Hubble parameters

at the beginning and ending points of the bouncing phase are $-\mathcal{H}_{con}/M_P \sim \mathcal{O}(10^{-4})$ and $\mathcal{H}_{exp}/M_P \sim \mathcal{O}(10^{-5})$ respectively. We plot the primordial power spectra with limits from P18 data sets, as shown in FIG. 1. Unlike ΛCDM (PL), in the ΛCDM (BI) model, the power spectrum presents some oscillating behaviors at large scales (small $k$). Moreover, there is also a suppression at even larger scales, making the spectrum blue-tilted. These are typical behaviors in the BI scenario [8, 13–15]. While the former is probably due to the inside-horizon effects during the bounce process, the latter is because of the horizon exit in the contracting phase, which changes the initial condition of the expanding phase.

### B. Cosmological Parameters

The Hubble and $S_8$ tensions are two of the most serious cosmological tensions. Usually, the standard cosmological model is defined by six parameters, which are taken to be $\{\omega_b, \omega_{cdm}, \theta_s, \tau_{reio}, A_s, n_s\}$, if one assumes a PL primordial power spectrum like Eq. (7). The first two parameters describe the densities of baryon and cold dark matter which are given by the parameters $\omega_b = \Omega_b h^2$ and $\omega_{cdm} = \Omega_{cdm} h^2$. $\theta_s$ is the angular scale of the sound horizon and $\tau$ is the optical depth due to reionization. However, in our BI model, the primordial power spectrum is described by five parameters in TABLE I and $\{A_s, n_s\}$ can be derived from other parameters numerically by CLASS. Thus there are nine free parameters in the BI scenario based on ΛCDM (BI) model or ten parameters if we take part in $A_L$ as an extended parameter in ΛCDM (BI) + $A_L$ model, as shown in TABLE II.

| Params | P18 (BI) | P18 (BI+$A_L$) | P18+SPT3G (BI) | P18+SPT3G (BI+$A_L$) |
|---|---|---|---|---|
| $\boldsymbol{10^2\omega_b}$ | $2.254^{+0.013}_{-0.015}$ | $2.269 \pm 0.015$ | $2.252 \pm 0.013$ | $2.259 \pm 0.013$ |
| $\boldsymbol{\omega_{cdm}}$ | $0.11717 \pm 0.00092$ | $0.1155 \pm 0.0010$ | $0.11622 \pm 0.00083$ | $0.11490 \pm 0.00096$ |
| $\boldsymbol{100\theta_s}$ | $1.04209 \pm 0.00028$ | $1.04220 \pm 0.00029$ | $1.04218 \pm 0.00026$ | $1.04211 \pm 0.00025$ |
| $\boldsymbol{\tau_{reio}}$ | $0.0616 \pm 0.0072$ | $0.0492 \pm 0.0081$ | $0.0645 \pm 0.0075$ | $0.0506 \pm 0.0077$ |
| $\boldsymbol{A_L}$ | | $1.128 \pm 0.038$ | | $1.116 \pm 0.036$ |
| $\boldsymbol{\Omega_m}$ | $0.2983 \pm 0.0055$ | $0.2885 \pm 0.0060$ | $0.2931 \pm 0.0048$ | $0.2861 \pm 0.0055$ |
| $\boldsymbol{H_0}$ | $68.60^{+0.40}_{-0.45}$ | $69.38 \pm 0.49$ | $68.96 \pm 0.38$ | $69.49 \pm 0.45$ |
| $\boldsymbol{S_8}$ | $0.806 \pm 0.011$ | $0.774 \pm 0.014$ | $0.797 \pm 0.010$ | $0.771^{+0.013}_{-0.012}$ |
| $\boldsymbol{10^9 A_s}$ | $2.115^{+0.028}_{-0.031}$ | $2.051 \pm 0.035$ | $2.119 \pm 0.032$ | $2.053 \pm 0.032$ |
| $\boldsymbol{n_s}$ | $0.9802 \pm 0.0043$ | $0.9809 \pm 0.0046$ | $0.9839 \pm 0.0042$ | $0.9841^{+0.0045}_{-0.0040}$ |

TABLE II: Cosmological parameters (Mean and 68% limits) of ΛCDM (BI)(with $A_L = 1$) and the extended model ΛCDM (BI) + $A_L$.

As demonstrated in TABLE II, the Hubble parameters in the extended ΛCDM (BI) + $A_L$ model are larger than the one in ΛCDM (BI). There are roughly $1\sigma$ difference of $H_0$ and $2\sigma$ difference of $S_8$ between the ΛCDM (BI) + $A_L$ and ΛCDM (BI). Therefore, although there is $2\sigma$ tension in $S_8$ in the ΛCDM (BI) model, there will be no tension in the extended ΛCDM (BI) + $A_L$ model. Another parameter with significant differences between the two

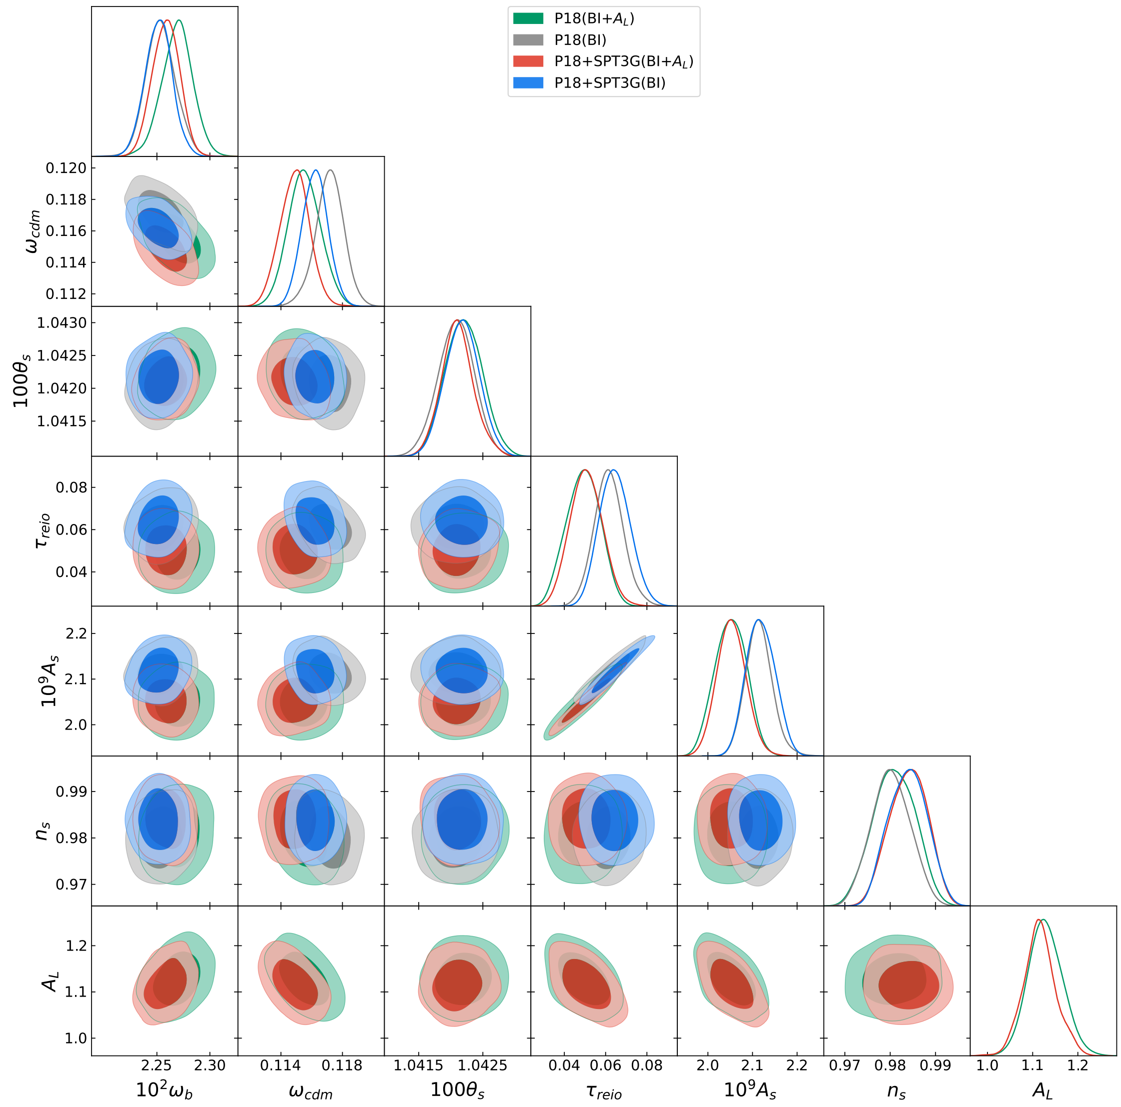


FIG. 2: Cosmological parameters with data sets P18 and P18+SPT3G based on $\Lambda$CDM (BI) model and the extended $\Lambda$CDM (BI) + $A_L$ model.

models is the optical depth of reionization $\tau_{reio}$. Our numerical analyses show a strong degeneracy between $\tau_{reio}$ and $A_L$.

### C. CMB Lensing Anomaly

Both reionization and weak lensing of the CMB can wash out the primordial anisotropies[16–21]. Thus there is a strong degeneracy between optical depth $\tau_{reio}$ and gravitational lensing amplitude $A_L$. Our results give that $\tau_{reio}$ is approximately equal to 0.06 in $\Lambda$CDM (BI) model(with $A_L = 1$) and approximately equal to 0.05 in $\Lambda$CDM (BI) + $A_L$ model (with $A_L \approx 1.13$), as shown in TABLE II.

We guess the CMB lensing anomaly may be caused by the degeneracy between $\tau_{reio}$ and $A_L$. So we add a Gaussian prior of the optical depth with $\tau_{prior} = 0.088 \pm 0.015$ from WAMP

9-year results [22] as a new likelihood artificially. Our result implies that data sets with a prior of optical depth will give a larger $\tau_{reio}$ that is approximately equal to 0.058 and the smaller $A_L$ that is approximately equal to 1.10, which will ulteriorly remit the CMB lensing anomaly. By the way, the cosmological tensions are not aggravated when we add this prior, as shown in TABLE III

| Params | P18+$\tau_{\rm prior}$ | P18+SPT3G+$\tau_{\rm prior}$ |
|---|---|---|
| $\boldsymbol{\tau_{reio}}$ | $0.0577 \pm 0.0076$ | $0.0579 \pm 0.0073$ |
| $\boldsymbol{A_L}$ | $1.100 \pm 0.040$ | $1.102 \pm 0.034$ |
| $\boldsymbol{\Omega_m}$ | $0.2913^{+0.0050}_{-0.0061}$ | $0.2857 \pm 0.0050$ |
| $\boldsymbol{H_0}$ | $69.17^{+0.49}_{-0.44}$ | $69.57 \pm 0.42$ |
| $\boldsymbol{S_8}$ | $0.787 \pm 0.014$ | $0.776 \pm 0.012$ |
| $\boldsymbol{10^{-9}A_s}$ | $2.088 \pm 0.037$ | $2.081 \pm 0.030$ |
| $\boldsymbol{n_s}$ | $0.9789 \pm 0.0041$ | $0.9841 \pm 0.0041$ |

TABLE III: Cosmological parameters (Mean and 68% limits) of ΛCDM (BI) + $A_L$ model with P18 and P18+SPT3G data sets by adding the Gaussian prior $\tau_{prior} = 0.088 \pm 0.015$ [22].


[1] J. K. Erickson, D. H. Wesley, P. J. Steinhardt, and N. Turok, Phys. Rev. D **69**, 063514 (2004), arXiv:hep-th/0312009 .

[2] J. Khoury, B. A. Ovrut, P. J. Steinhardt, and N. Turok, Phys. Rev. D **64**, 123522 (2001), arXiv:hep-th/0103239 .

[3] T. Qiu, X. Gao, and E. N. Saridakis, Phys. Rev. D **88**, 043525 (2013), arXiv:1303.2372 [astro-ph.CO] .

[4] B. Xue and P. J. Steinhardt, Phys. Rev. Lett. **105**, 261301 (2010), arXiv:1007.2875 [hep-th] .

[5] B. Xue and P. J. Steinhardt, Phys. Rev. D **84**, 083520 (2011), arXiv:1106.1416 [hep-th] .

[6] Y.-F. Cai, T. Qiu, Y.-S. Piao, M. Li, and X. Zhang, JHEP **10**, 071, arXiv:0704.1090 [gr-qc] .

[7] T. Qiu and Y.-T. Wang, JHEP **04**, 130, arXiv:1501.03568 [astro-ph.CO] .

[8] S. Ni, H. Li, T. Qiu, W. Zheng, and X. Zhang, Eur. Phys. J. C **78**, 608 (2018), arXiv:1707.05570 [astro-ph.CO] .

[9] Y. Cai, Y. Wan, H.-G. Li, T. Qiu, and Y.-S. Piao, JHEP **01**, 090, arXiv:1610.03400 [gr-qc] .

[10] Y. Cai, H.-G. Li, T. Qiu, and Y.-S. Piao, Eur. Phys. J. C **77**, 369 (2017), arXiv:1701.04330 [gr-qc] .

[11] T. Qiu, J. Evslin, Y.-F. Cai, M. Li, and X. Zhang, JCAP **10**, 036, arXiv:1108.0593 [hep-th] .

[12] N. Aghanim et al. (Planck), Astron. Astrophys. **641**, A6 (2020), [Erratum: Astron.Astrophys. 652, C4 (2021)], arXiv:1807.06209 [astro-ph.CO] .

[13] Y.-S. Piao, B. Feng, and X.-m. Zhang, Phys. Rev. D **69**, 103520 (2004), arXiv:hep-th/0310206 .

[14] Z.-G. Liu, Z.-K. Guo, and Y.-S. Piao, Phys. Rev. D **88**, 063539 (2013), arXiv:1304.6527 [astro-ph.CO] .

[15] T. Qiu and M. Zhu, (2024), arXiv:2408.06582 [gr-qc] .

[16] E. Calabrese, A. Slosar, A. Melchiorri, G. F. Smoot, and O. Zahn, Phys. Rev. D **77**, 123531 (2008), arXiv:0803.2309 [astro-ph] .

[17] G. Domènech and M. Kamionkowski, JCAP **11**, 040, arXiv:1905.04323 [astro-ph.CO] .

[18] G. E. Addison, C. L. Bennett, M. Halpern, G. Hinshaw, and J. L. Weiland, (2023), arXiv:2310.03127 [astro-ph.CO] .

[19] W. Giarè, E. Di Valentino, and A. Melchiorri, Phys. Rev. D **109**, 103519 (2024), arXiv:2312.06482 [astro-ph.CO] .

[20] G. Domènech, X. Chen, M. Kamionkowski, and A. Loeb, JCAP **10**, 005, arXiv:2005.08998 [astro-ph.CO] .

[21] D. K. Hazra, A. Antony, and A. Shafieloo, JCAP **08** (08), 063, arXiv:2201.12000 [astro-ph.CO] .

[22] G. Hinshaw et al. (WMAP), Astrophys. J. Suppl. **208**, 19 (2013), arXiv:1212.5226 [astro-ph.CO] .
